# Supplementary material for: The Plateau-Rayleigh instability in solids is a simple phase separation
Source: arXiv:1701.03832 ancillary file (2017-01-13)
Supplement: Supplementary file 1 [file theoretical_SI.pdf]

# The Plateau-Rayleigh instability in solids is a simple phase separation: Theoretical Supplement

Chen Xuan and John Biggins

We undertake a small-gradient expansion of the fields in a long elastic cylinder subject to surface tension and close to its point of instability, and thereby calculate the precise width of a domain wall.

We consider a long elastic cylinder, of radius $a$ and shear modulus $\mu$, subject to a surface tension $\gamma = \Gamma\mu a$. The cylinder is aligned along the $z$ axis of a cylindrical coordinate system and undergoes a uniaxial deformation that moves the material at $(R, \theta, Z)$ to $(r(R, Z), \theta, z(R, Z))$, leading to the (cylindrical-coordinate) deformation gradient

$$F = \begin{pmatrix} \frac{\partial r}{\partial R} & 0 & \frac{\partial r}{\partial Z} \\ 0 & r/R & 0 \\ \frac{\partial z}{\partial R} & 0 & \frac{\partial z}{\partial Z} \end{pmatrix}. \quad (1)$$

As in the main text, if the cylinder is subject to a tension $T$, its mechanical behavior is given by the minimum of the effective energy

$$E = \int \mathcal{E}\, dZ = \int \left( E_s + E_{el} - T \frac{\partial z}{\partial Z}\bigg|_{R=0} \right) dZ, \quad (2)$$

where the surface energy per unit length is

$$E_s = \Gamma a \mu 2\pi r(a, Z) \sqrt{\left(\frac{\partial r(a, Z)}{\partial Z}\right)^2 + \left(\frac{\partial z(a, Z)}{\partial Z}\right)^2}, \quad (3)$$

but the elastic energy per unit length must now include a pressure-field Lagrange multiplier to enforce volume conservation throughout the cylinder

$$E_{el} = \int_0^a \frac{1}{2}\mu \left[ \mathrm{Tr}\left(F \cdot F^T\right) + P(\mathrm{Det}\,(F) - 1)\right] 2\pi R \mathrm{d}R. \quad (4)$$

Introducing the PK1 stress $\sigma = \mu F + \mathrm{Det}\,(F)\, F^{-T} P$, we see that minimizing $E$ with respect to variations in $r, z$ leads to the familiar equations of elastic equilibrium inside the cylinder

$$\nabla\cdot\sigma = 0 \quad \Longrightarrow \quad \begin{cases} \sigma_{rR,R} + \sigma_{rZ,Z} + (\sigma_{rR} - \sigma_{\theta\theta})/R = 0, \\ \sigma_{zR,R} + \sigma_{zZ,Z} + \sigma_{zR}/R = 0, \end{cases} \quad (5)$$

and the boundary condition at the outer surface

$$\sigma \cdot (2\pi a \hat{\mathbf{r}}) = \begin{pmatrix} -\frac{\partial E_s}{\partial r} + \frac{d}{dZ}\frac{\partial E_s}{\partial r_{,Z}} \\ 0 \\ \frac{d}{dZ}\frac{\partial E_s}{\partial z_{,Z}} \end{pmatrix}, \quad (6)$$

where, for conciseness, we use comma-notation for partial derivatives. Finally, minimizing $E$ with respect to $P$ yields the expected condition of incompressibility,

$$\mathrm{Det}\,(F) = 1. \quad (7)$$

We know from the main text that instability first occurs at $\Gamma = \sqrt{32}$ in a homogeneously strained cylinder with $z = 2^{1/3}Z$ and $r = R/2^{1/6}$. Furthermore, just beyond the threshold for instability, $\Gamma = \sqrt{32} + \epsilon$, we expect variation in the $Z$ direction only over length scales $a/\sqrt{\epsilon}$, and strains no larger than $\mathcal{O}(\sqrt{\epsilon})$, so we can write the pressure and position fields as expansions in $\sqrt{\epsilon}$,

$$z = 2^{1/3}Z + a z_0\left(\tilde{Z}\right) + \sum_{i=1}^{\infty} \epsilon^{i/2} a z_i\left(\tilde{R}, \tilde{Z}\right) \quad (8)$$

$$r = \frac{R}{2^{1/6}} + \sum_{i=1}^{\infty} \epsilon^{i/2} a r_i\left(\tilde{R}, \tilde{Z}\right) \quad (9)$$

$$P = \mu P_0 + \sum_{i=1}^{\infty} \epsilon^{i/2} \mu p_i\left(\tilde{R}, \tilde{Z}\right), \quad (10)$$

where $\tilde{Z} \equiv \sqrt{\epsilon} z/a$ and $\tilde{R} \equiv R/a$ are dimensionless coordinates of order unity, and $p_i$, $z_i$ and $r_i$ are dimensionless functions, also of order unity. An important subtlety is the need to include a $z_0$ term in the expansion as, provided it does not depend upon $R$, it only generates an $\mathcal{O}(\sqrt{\epsilon})$ term in $F$. Indeed, comparing to the answer in the main text, we will later choose to write

$$z_{0,\tilde{Z}} = \frac{2^{7/12}}{\sqrt{3}} h\left(\tilde{Z}\right), \quad (11)$$

where $h$ is the function we are seeking, which varies between $\pm 1$ over the domain wall.

Our strategy is to substitute these series expansions into the bulk equations (eqns 5 and 7) and boundary conditions (eqn 6), and solve at each successive order in $\epsilon$ to properly characterize the sympathetic strains that accompany $z_0$.

Both $F$ and $\sigma$ can also be expanded in $\epsilon$,

$$F = \sum_{i=0}^{\infty} \epsilon^{i/2} F_i, \qquad \sigma = \sum_{i=0}^{\infty} \epsilon^{i/2} \sigma_i, \quad (12)$$

and the zeroth terms in $F$ and $\sigma$ are

$$F_0 = \begin{pmatrix} 2^{-1/6} & 0 & 0 \\ 0 & 2^{-1/6} & 0 \\ 0 & 0 & 2^{1/3} \end{pmatrix} \quad (13)$$

$$\frac{\sigma_0}{\mu} = \begin{pmatrix} 2^{-\frac{1}{6}} + 2^{\frac{1}{6}} P_0 & 0 & 0 \\ 0 & 2^{-\frac{1}{6}} + 2^{\frac{1}{6}} P_0 & 0 \\ 0 & 0 & 2^{\frac{1}{3}} + 2^{-\frac{1}{3}} P_0 \end{pmatrix}, \quad (14)$$

which already solve eqns 5 and 7 (the bulk equations) to zeroth order. Inspecting the expansions for $z$ and $r$, we see that $E_s = \Gamma a\mu 2\pi r z_{,Z} + \mathcal{O}(\epsilon^2)$, so the boundary conditions at $R = a$ can be written in much simpler form,

$$\sigma_{rR}/\mu = -\Gamma z_{,Z} + \mathcal{O}(\epsilon^{3/2}) \quad (15)$$

$$\sigma_{zR}/\mu = \Gamma r_{,Z} + \mathcal{O}(\epsilon^{5/2}), \quad (16)$$

and, to satisfy these to zeroth order, we require

$$P_0 = -\frac{9}{2^{1/3}}. \quad (17)$$

To solve at $\mathcal{O}(\sqrt{\epsilon})$ we first need the next term in $F$,

$$F_1 = \begin{pmatrix} r_{1,\tilde{R}} & 0 & 0 \\ 0 & r_1/\tilde{R} & 0 \\ z_{1,\tilde{R}} & 0 & z_{0,\tilde{Z}} \end{pmatrix}. \quad (18)$$

To satisfy the volume-conservation equation (eqn 7) at $\mathcal{O}(\sqrt{\epsilon})$ we require

$$2^{\frac{1}{6}} r_{1,\tilde{R}} + 2^{\frac{1}{6}} \frac{r_1}{\tilde{R}} + 2^{-\frac{1}{3}} z_{0,\tilde{Z}} = 0, \quad (19)$$

and hence

$$r_1(\tilde{R}, \tilde{Z}) = -\frac{\tilde{R}}{2\sqrt{2}} z_{0,\tilde{Z}}, \quad (20)$$

where we have set the complimentary function, $c(\tilde{Z})/\tilde{R}$, to zero as otherwise it diverges at the center of the cylinder. The next order in the stress is

$$\frac{\sigma_1}{\mu} = p_1 F_0^{-1} + \begin{pmatrix} -\frac{5}{\sqrt{2}} z_{0,\tilde{Z}} & 0 & \frac{9}{\sqrt{2}} z_{1,\tilde{R}} \\ 0 & -\frac{5}{\sqrt{2}} z_{0,\tilde{Z}} & 0 \\ z_{1,\tilde{R}} & 0 & \frac{11}{2} z_{0,\tilde{Z}} \end{pmatrix}.$$

Substituting this into the mechanical equilibrium equations (eqn 5), remembering that $\frac{\partial}{\partial Z} = \frac{\sqrt{\epsilon}}{a}\frac{\partial}{\partial \tilde{Z}}$ and $\frac{\partial}{\partial R} = \frac{1}{a}\frac{\partial}{\partial \tilde{R}}$, we see that at $\mathcal{O}(\sqrt{\epsilon})$, the first equation simplifies to $p_{1,\tilde{R}} = 0$, requiring

$$p_1(\tilde{R}, \tilde{Z}) = p_1(\tilde{Z}), \quad (21)$$

while the second reduces to $z_{1,\tilde{R}\tilde{R}} + z_{1,\tilde{R}}/\tilde{R} = 0$, requiring

$$z_1(\tilde{R}, \tilde{Z}) = z_1(\tilde{Z}), \quad (22)$$

where we have again set the complimentary function, $c(\tilde{Z})\log(\tilde{R})$ to zero. Similarly, expanding the boundary conditions to $\mathcal{O}(\sqrt{\epsilon})$, eqn 16 is already satisfied, but eqn 15 is an algebraic equation for $p_1$ requiring

$$p_1(\tilde{Z}) = -\frac{3}{2^{2/3}} z_{0,\tilde{Z}}. \quad (23)$$

To solve at $\mathcal{O}(\epsilon)$ we first need the next term in $F$,

$$F_2 = \begin{pmatrix} r_{2,\tilde{R}} & 0 & r_{1,\tilde{Z}} \\ 0 & r_2/\tilde{R} & 0 \\ z_{2,\tilde{R}} & 0 & z_{1,\tilde{Z}} \end{pmatrix}. \quad (24)$$

To satisfy the volume-conservation equation (eqn 7) at $\mathcal{O}(\epsilon)$ we require

$$2^{\frac{1}{6}} r_{2,\tilde{R}} + 2^{\frac{1}{6}} \frac{r_2}{\tilde{R}} + 2^{-\frac{1}{3}} z_{1,\tilde{Z}} - \frac{3}{4 \times 2^{2/3}} z_{0,\tilde{Z}}^2 = 0, \quad (25)$$

which is solved by

$$r_2(\tilde{R}, \tilde{Z}) = \frac{3\tilde{R}}{8 \times 2^{5/6}} z_{0,\tilde{Z}}^2 - \frac{\tilde{R}}{2\sqrt{2}} z_{1,\tilde{Z}}. \quad (26)$$

The next term in $\sigma$ then simplifies to

$$\frac{\sigma_2}{\mu} = p_2 F_0^{-1} + \begin{pmatrix} -5 z_{1,\tilde{Z}}/\sqrt{2} & 0 & \ldots \\ 0 & -5 z_{1\tilde{Z}}/\sqrt{2} & 0 \\ z_{2,\tilde{R}} - \frac{9}{4}\tilde{R} z_{0,\tilde{Z}\tilde{Z}} & 0 & \ldots \end{pmatrix},$$

where we have not displayed the $rZ$ and $zZ$ entries since they do not enter the equations at $\mathcal{O}(\epsilon)$. Expanding the mechanical equilibrium equations (eqn 5) to $\mathcal{O}(\epsilon)$, first equation simplifies to $p_{2,\tilde{R}} = 0$, requiring

$$p_2(\tilde{R}, \tilde{Z}) = p_2(\tilde{Z}), \quad (27)$$

and the second simplifies to

$$z_{2,\tilde{R}\tilde{R}} - \frac{9}{4} z_{0,\tilde{Z}\tilde{Z}} + \frac{11}{2} z_{0,\tilde{Z}\tilde{Z}} - \frac{3}{2} z_{0,\tilde{Z}\tilde{Z}} + \frac{z_{2,\tilde{R}}}{\tilde{R}} - \frac{9}{4} z_{0,\tilde{Z}\tilde{Z}} = 0, \quad (28)$$

which we can solve to find

$$z_2(\tilde{R}, \tilde{Z}) = C(\tilde{Z}) + \frac{1}{8}\tilde{R}^2 z_{0,\tilde{Z}\tilde{Z}}. \quad (29)$$

Expanding out the boundary conditions to $\mathcal{O}(\epsilon)$, eqn 15 is an algebraic equation for $p_2$ that requires

$$p_2(\tilde{Z}) = -2^{1/6} - \frac{3}{2^{2/3}} z_{1,\tilde{Z}}, \quad (30)$$

while eqn 16 is already satisfied.

Recalling from the main text that instability occurs when the tension is,

$$T = \frac{\pi\mu a^2}{2^{2/3}} \left(9 + \sqrt{2}\epsilon + \mathcal{O}(\epsilon^2)\right), \quad (31)$$

and writing

$$z_{0,\tilde{Z}} = \frac{2^{7/12}}{\sqrt{3}} h\left(\tilde{Z}\right), \quad (32)$$

we can now expand out the total energy per unit length (eqn 2) to $\mathcal{O}(\epsilon^2)$, to get

$$\frac{\mathcal{E}}{\pi\mu a^2} = \frac{9}{\sqrt[3]{2}} + 2^{\frac{1}{6}}\pi a^2\mu\epsilon + \left(\frac{25h''}{16\sqrt[12]{2}\sqrt{3}} + c_1\right)\epsilon^{3/2} + \frac{1}{12\sqrt[3]{2}}\left(h^2\left(h^2 - 2\right) - 2\sqrt{2}hh'' + \frac{17}{4\sqrt{2}}h'^2 + c_2\right)\epsilon^2 + \mathcal{O}(\epsilon^{5/2}), \quad (33)$$

where $c_1$ and $c_2$ are quite complicated expressions involving higher order fields, but do not contain any $h$ dependence. The above expression is the exact version of the approximate eqn 13 in the main text. We note that one would naively expect cross terms between $z_0$ ( which generates $\mathcal{O}(\sqrt{\epsilon})$ stress/strains) and the $z_3$, $r_3$, $p_3$ fields (which generate $\mathcal{O}(\epsilon^{3/2})$ stress/strains) at $\mathcal{O}(\epsilon^2)$ in $\mathcal{E}$, but upon actually doing the expansion, we find these terms vanish identically; such cancelation is actually expected since the coefficient of such cross-terms would be the curvature (second derivative) of the energy at $\epsilon = 0$, which is zero since we are expanding about the point of instability. Minimizing with respect to variations in $h$, the $\mathcal{O}(\epsilon^{3/2})$ term is an exact derivative, so it does not contribute, but minimizing the $\mathcal{O}(\epsilon^2)$ term gives:

$$4h\left(h^2-1\right) = \frac{33}{2\sqrt{2}}h'', \tag{34}$$

which is solved by the domain wall taking the form

$$\begin{aligned} h(\tilde{Z}) &= \tanh\left(\frac{2^{5/4}\tilde{Z}}{\sqrt{33}}\right) \\ \Longrightarrow h(Z) &= \tanh\left(\frac{2^{5/4}\sqrt{\epsilon}}{\sqrt{33}a}Z\right). \end{aligned} \tag{35}$$

This is almost identical to the approximate result in the main text, but with a characteristic width for the domain wall smaller by a factor of $\sqrt{34/33}$.
